# Supplementary material for: Unnatural Instructions: Tuning Language Models with (Almost) No Human Labor
Source: arXiv:2212.09689 source file (2022-12-19)
Supplement: Supplementary file 1 [file additional_inputs_prompt.tex]

\definecolor{modelcolor}{RGB}{147,75,201}

\definecolor{promptcolor}{cmyk}{1,0.3968,0,0.2588} 
% \definecolor{modelcolor}{cmyk}{0.1127,0.6690,0,0.4431}
% \definecolor{modelcolor}{cmyk}{0,0.6175,0.8848,0.1490}

\begin{figure}
    \centering
    \small
    \begin{tabularx}{\linewidth}{@{}X@{}}
    \toprule
    \textcolor{promptcolor}{Example 1}\\
    \textcolor{promptcolor}{Instruction: }You are given a science question (easy-level) and four answer options (associated with ``A'', ``B'', ``C'', ``D''). Your task is to find the correct answer...\\
    \\
    \textcolor{promptcolor}{Three inputs:}\\
    \textcolor{promptcolor}{Input 1: }Which part of a bicycle BEST moves in a circle? (A) Seat (B) Frame (C) Foot pedal (D) Kickstand\\
    \textcolor{promptcolor}{Input 2: }Which measurement represents...\\
    \textcolor{promptcolor}{Input 3: }Which of these is a nonliving part...\\
    My college roommate asked me what this article means: "{INPUT}". So I recapped it in layman's terms:\\
    \\
    \textcolor{promptcolor}{Example 2}\\
    \textcolor{promptcolor}{Instruction: }You are given a negative review and your task is to convert it to a positive review by one or more making minimal changes. Avoid changing the context of the review.\\
    \\
    \textcolor{promptcolor}{Three inputs:}\\
    \textcolor{promptcolor}{Input 1: }we stood there in shock, because...\\
    \textcolor{promptcolor}{Input 2: }very bad viewing alternative.\\
    \textcolor{promptcolor}{Input 3: }horrible! very bad acting.\\
    \\
    \textcolor{promptcolor}{Example 3}\\
    \textcolor{promptcolor}{Instruction: }You need to output the meaning of an idiom. An idiom is a phrase whose meaning cannot be understood from the meanings of the individual words that make it up.\\
    \\
    \textcolor{promptcolor}{Three inputs:}\\
    \textcolor{promptcolor}{Input 1: }Text: I have bigger fish to fry.\\
    \textcolor{modelcolor}{Input 2: Text: That'll be the day!}\\
    \textcolor{modelcolor}{Input 3: Text: I'm all ears.}\\
    \bottomrule
    \end{tabularx}
    \caption{The multiple inputs generation prompt. \textcolor{promptcolor}{Blue}: Two few-shot demonstrations of instructions and three corresponding inputs. Example 3 contains an instruction and one input example, and the model should suggest two additional inputs. \textcolor{modelcolor}{Purple}: An example of model-generated additional inputs.}
    \label{fig:multiple_inputs_prompt}
\end{figure}
